# Supplementary material for: Facebook Ads Monitor: An Independent Auditing System for Political Ads on Facebook
Source: arXiv:2001.10581 source file (2020-01-31)
Supplement: Supplementary file 1 [file appendix.tex]

%\appendix
\section*{Appendix}

\begingroup
\setlength{\tabcolsep}{4pt} % Default value: 6pt
 % Default value: 1

\begin{table}[!hbt]
  
  \tiny
  \centering
  \caption{2-classes experiments results with 4 machine learning approaches}
  
  \label{tab:result_table}
    \begin{tabular}{|c|r|c|c|c|c|c|c|c|c|c}
    	
    \hline
    \multirow{2}[2]{*}{\textbf{Input}} & \multicolumn{1}{c|}{\multirow{2}[2]{*}{\textbf{Approach}}} & \multirow{2}[2]{*}{\textbf{Accuracy}} & \multicolumn{3}{c|}{\textbf{Political}} & \multicolumn{3}{c|}{\textbf{Non Political}} & \multirow{2}[2]{*}{\textbf{Macro-F1}} \\
    
          & \multicolumn{1}{c|}{} &       & \multicolumn{1}{c}{\textbf{P}} & \multicolumn{1}{c}{\textbf{R}} & \textbf{F1} & \multicolumn{1}{c}{\textbf{P}} & \multicolumn{1}{c}{\textbf{R}} & \textbf{F1} & \\

S1 & \multicolumn{1}{l|}{Mult.NB} & $0.48 (\pm 0.02)$ & $0.03 (\pm 0.00)$ & $0.78 (\pm 0.10)$ & $0.06 (\pm 0.01)$ & $0.99 (\pm 0.01)$ & $0.48 (\pm 0.02)$ & $0.64 (\pm 0.02)$ & $0.35 (\pm 0.01)$ \\
 & \multicolumn{1}{l|}{CNN} & $0.85 (\pm 0.04)$ & $0.12 (\pm 0.03)$ & $0.81 (\pm 0.14)$ & $0.20 (\pm 0.04)$ & $0.99 (\pm 0.00)$ & $0.85 (\pm 0.04)$ & $0.92 (\pm 0.02)$ & $0.56 (\pm 0.03)$ \\
 & \multicolumn{1}{l|}{logistic} & $0.91 (\pm 0.02)$ & $0.17 (\pm 0.04)$ & $0.75 (\pm 0.15)$ & $0.28 (\pm 0.05)$ & $0.99 (\pm 0.00)$ & $0.91 (\pm 0.02)$ & $0.95 (\pm 0.01)$ & $0.61 (\pm 0.03)$ \\
 & \multicolumn{1}{l|}{gdboosting} & $0.87 (\pm 0.01)$ & $0.12 (\pm 0.01)$ & $0.75 (\pm 0.10)$ & $0.21 (\pm 0.02)$ & $0.99 (\pm 0.00)$ & $0.87 (\pm 0.01)$ & $0.93 (\pm 0.00)$ & $0.57 (\pm 0.01)$ \\
 \hline 
S1 S2 & \multicolumn{1}{l|}{Mult.NB} & \boldmath$0.98 (\pm 0.00)$ & \boldmath$0.53 (\pm 0.13)$ & \boldmath$0.59 (\pm 0.14)$ & \boldmath$0.55 (\pm 0.11)$ & \boldmath$0.99 (\pm 0.00)$ & \boldmath$0.99 (\pm 0.00)$ & \boldmath$0.99 (\pm 0.00)$ & \boldmath$0.77 (\pm 0.05)$ \\
 & \multicolumn{1}{l|}{CNN} & \boldmath$0.98 (\pm 0.01)$ & \boldmath$0.63 (\pm 0.12)$ & \boldmath$0.54 (\pm 0.11)$ & \boldmath$0.58 (\pm 0.11)$ & \boldmath$0.99 (\pm 0.00)$ & \boldmath$0.99 (\pm 0.00)$ & \boldmath$0.99 (\pm 0.00)$ & \boldmath$0.79 (\pm 0.06)$ \\
 & \multicolumn{1}{l|}{logistic} & \boldmath$0.98 (\pm 0.01)$ & \boldmath$0.58 (\pm 0.21)$ & \boldmath$0.47 (\pm 0.12)$ & \boldmath$0.51 (\pm 0.11)$ & \boldmath$0.99 (\pm 0.00)$ & \boldmath$0.99 (\pm 0.01)$ & \boldmath$0.99 (\pm 0.00)$ & \boldmath$0.75 (\pm 0.06)$ \\
 & \multicolumn{1}{l|}{gdboosting} & $0.97 (\pm 0.00)$ & $0.44 (\pm 0.05)$ & $0.48 (\pm 0.04)$ & $0.46 (\pm 0.04)$ & $0.99 (\pm 0.00)$ & $0.99 (\pm 0.00)$ & $0.99 (\pm 0.00)$ & $0.72 (\pm 0.02)$ \\
 \hline
S1 S2 S3 & \multicolumn{1}{l|}{Mult.NB} & $0.91 (\pm 0.01)$ & $0.20 (\pm 0.04)$ & $0.92 (\pm 0.12)$ & $0.33 (\pm 0.05)$ & $1.00 (\pm 0.00)$ & $0.91 (\pm 0.01)$ & $0.95 (\pm 0.00)$ & $0.64 (\pm 0.03)$ \\
 & \multicolumn{1}{l|}{CNN} & $0.92 (\pm 0.01)$ & $0.20 (\pm 0.03)$ & $0.90 (\pm 0.07)$ & $0.33 (\pm 0.04)$ & $1.00 (\pm 0.00)$ & $0.92 (\pm 0.01)$ & $0.96 (\pm 0.01)$ & $0.64 (\pm 0.02)$ \\
 & \multicolumn{1}{l|}{logistic} & $0.89 (\pm 0.01)$ & $0.16 (\pm 0.03)$ & $0.94 (\pm 0.05)$ & $0.27 (\pm 0.04)$ & $1.00 (\pm 0.00)$ & $0.88 (\pm 0.01)$ & $0.94 (\pm 0.01)$ & $0.61 (\pm 0.02)$ \\
 & \multicolumn{1}{l|}{gdboosting} & $0.83 (\pm 0.01)$ & $0.11 (\pm 0.01)$ & $0.92 (\pm 0.14)$ & $0.20 (\pm 0.02)$ & $1.00 (\pm 0.00)$ & $0.83 (\pm 0.01)$ & $0.91 (\pm 0.01)$ & $0.56 (\pm 0.01)$ \\
 \hline 
S1 S3 & \multicolumn{1}{l|}{Mult.NB} & $0.91 (\pm 0.02)$ & $0.20 (\pm 0.06)$ & $0.91 (\pm 0.12)$ & $0.33 (\pm 0.08)$ & $1.00 (\pm 0.00)$ & $0.91 (\pm 0.02)$ & $0.95 (\pm 0.01)$ & $0.64 (\pm 0.05)$ \\
 & \multicolumn{1}{l|}{CNN} & $0.92 (\pm 0.02)$ & $0.21 (\pm 0.06)$ & $0.89 (\pm 0.07)$ & $0.34 (\pm 0.08)$ & $1.00 (\pm 0.00)$ & $0.92 (\pm 0.02)$ & $0.96 (\pm 0.01)$ & $0.65 (\pm 0.04)$ \\
 & \multicolumn{1}{l|}{logistic} & $0.89 (\pm 0.01)$ & $0.16 (\pm 0.03)$ & $0.94 (\pm 0.05)$ & $0.28 (\pm 0.04)$ & $1.00 (\pm 0.00)$ & $0.88 (\pm 0.01)$ & $0.94 (\pm 0.01)$ & $0.61 (\pm 0.02)$ \\
 & \multicolumn{1}{l|}{gdboosting} & $0.85 (\pm 0.04)$ & $0.13 (\pm 0.05)$ & $0.92 (\pm 0.10)$ & $0.22 (\pm 0.07)$ & $1.00 (\pm 0.00)$ & $0.85 (\pm 0.05)$ & $0.92 (\pm 0.03)$ & $0.57 (\pm 0.05)$ \\
 \hline
S2 & \multicolumn{1}{l|}{Mult.NB} & $0.92 (\pm 0.02)$ & $0.21 (\pm 0.05)$ & $0.88 (\pm 0.09)$ & $0.34 (\pm 0.07)$ & $1.00 (\pm 0.00)$ & $0.92 (\pm 0.02)$ & $0.96 (\pm 0.01)$ & $0.65 (\pm 0.04)$ \\
 & \multicolumn{1}{l|}{CNN} & \boldmath$0.98 (\pm 0.01)$ & \boldmath$0.83 (\pm 0.19)$ & \boldmath$0.39 (\pm 0.17)$ & \boldmath$0.52 (\pm 0.19)$ & \boldmath$0.99 (\pm 0.00)$ & \boldmath$1.00 (\pm 0.00)$ & \boldmath$0.99 (\pm 0.00)$ & \boldmath$0.76 (\pm 0.10)$ \\
 & \multicolumn{1}{l|}{logistic} & $0.98 (\pm 0.00)$ & $0.68 (\pm 0.32)$ & $0.15 (\pm 0.09)$ & $0.25 (\pm 0.14)$ & $0.98 (\pm 0.00)$ & $1.00 (\pm 0.00)$ & $0.99 (\pm 0.00)$ & $0.62 (\pm 0.07)$ \\
 & \multicolumn{1}{l|}{gdboosting} & $0.97 (\pm 0.01)$ & $0.33 (\pm 0.26)$ & $0.22 (\pm 0.23)$ & $0.25 (\pm 0.22)$ & $0.98 (\pm 0.01)$ & $0.99 (\pm 0.01)$ & $0.99 (\pm 0.00)$ & $0.62 (\pm 0.11)$ \\
 \hline
S2 S3 & \multicolumn{1}{l|}{Mult.NB} & $0.92 (\pm 0.01)$ & $0.21 (\pm 0.04)$ & $0.90 (\pm 0.12)$ & $0.34 (\pm 0.06)$ & $1.00 (\pm 0.00)$ & $0.92 (\pm 0.01)$ & $0.96 (\pm 0.01)$ & $0.65 (\pm 0.03)$ \\
 & \multicolumn{1}{l|}{CNN} & $0.91 (\pm 0.02)$ & $0.19 (\pm 0.05)$ & $0.90 (\pm 0.05)$ & $0.31 (\pm 0.06)$ & $1.00 (\pm 0.00)$ & $0.91 (\pm 0.02)$ & $0.95 (\pm 0.01)$ & $0.63 (\pm 0.03)$ \\
 & \multicolumn{1}{l|}{logistic} & $0.88 (\pm 0.01)$ & $0.15 (\pm 0.02)$ & $0.95 (\pm 0.07)$ & $0.26 (\pm 0.03)$ & $1.00 (\pm 0.00)$ & $0.88 (\pm 0.01)$ & $0.93 (\pm 0.00)$ & $0.60 (\pm 0.02)$ \\
 & \multicolumn{1}{l|}{gdboosting} & $0.84 (\pm 0.04)$ & $0.12 (\pm 0.05)$ & $0.93 (\pm 0.07)$ & $0.21 (\pm 0.08)$ & $1.00 (\pm 0.00)$ & $0.83 (\pm 0.04)$ & $0.91 (\pm 0.03)$ & $0.56 (\pm 0.05)$ \\
 \hline
S3 & \multicolumn{1}{l|}{Mult.NB} & $0.92 (\pm 0.01)$ & $0.21 (\pm 0.05)$ & $0.90 (\pm 0.12)$ & $0.34 (\pm 0.06)$ & $1.00 (\pm 0.00)$ & $0.92 (\pm 0.01)$ & $0.96 (\pm 0.01)$ & $0.65 (\pm 0.03)$ \\
 & \multicolumn{1}{l|}{CNN} & $0.92 (\pm 0.01)$ & $0.21 (\pm 0.05)$ & $0.89 (\pm 0.07)$ & $0.34 (\pm 0.07)$ & $1.00 (\pm 0.00)$ & $0.92 (\pm 0.02)$ & $0.96 (\pm 0.01)$ & $0.65 (\pm 0.04)$ \\
 & \multicolumn{1}{l|}{logistic} & $0.88 (\pm 0.01)$ & $0.15 (\pm 0.02)$ & $0.95 (\pm 0.07)$ & $0.27 (\pm 0.03)$ & $1.00 (\pm 0.00)$ & $0.88 (\pm 0.01)$ & $0.93 (\pm 0.00)$ & $0.60 (\pm 0.02)$ \\
 & \multicolumn{1}{l|}{gdboosting} & $0.82 (\pm 0.01)$ & $0.11 (\pm 0.02)$ & $0.93 (\pm 0.08)$ & $0.20 (\pm 0.03)$ & $1.00 (\pm 0.00)$ & $0.82 (\pm 0.01)$ & $0.90 (\pm 0.01)$ & $0.55 (\pm 0.02)$ \\
 \hline
    \end{tabular}%
  \label{tab:tabelao2}%
\end{table}%

\begin{longtable}{|c|c|c|c|c|c|c|c|}
 \caption{Training Metrics.} \label{tab:long} \\ \hline

\multirow{2}{*}{Model}     & \multirow{2}{*}{Source} & \multicolumn{2}{c|}{Precision} & \multicolumn{2}{c|}{Recall} & \multicolumn{2}{c|}{F1-score}  \\ 
  & & Mean & Std & Mean & Std & Mean & Std \\ \hline
Mult.NB & S4 & $0.860$ & $\pm0.016$ & $0.809$ & $\pm0.025$ & $0.802$ & $\pm0.027$ \\ \hline
Svm & S4 & $0.929$ & $\pm0.020$ & $0.928$ & $\pm0.021$ & $0.928$ & $\pm0.021$ \\ \hline
Logistic & S4 & $0.928$ & $\pm0.022$ & $0.928$ & $\pm0.023$ & $0.928$ & $\pm0.023$ \\ \hline
Gdboosting & S4 & $0.909$ & $\pm0.019$ & $0.909$ & $\pm0.021$ & $0.909$ & $\pm0.020$ \\ \hline
Random forest & S4 & $0.917$ & $\pm0.026$ & $0.917$ & $\pm0.027$ & $0.914$ & $\pm0.028$ \\ \hline
Mult.NB & S3 & $0.705$ & $\pm0.080$ & $0.683$ & $\pm0.078$ & $0.673$ & $\pm0.085$ \\ \hline
Svm & S3 & $0.862$ & $\pm0.080$ & $0.859$ & $\pm0.079$ & $0.857$ & $\pm0.079$ \\ \hline
Logistic & S3 & $0.773$ & $\pm0.107$ & $0.754$ & $\pm0.088$ & $0.738$ & $\pm0.090$ \\ \hline
Gdboosting & S3 & $0.839$ & $\pm0.107$ & $0.832$ & $\pm0.115$ & $0.838$ & $\pm0.120$ \\ \hline
Random forest & S3 & $0.845$ & $\pm0.111$ & $0.837$ & $\pm0.123$ & $0.828$ & $\pm0.138$ \\ \hline
Mult.NB & S2 & $0.849$ & $\pm0.040$ & $0.799$ & $\pm0.069$ & $0.791$ & $\pm0.076$ \\ \hline
Svm & S2 & $0.899$ & $\pm0.064$ & $0.898$ & $\pm0.065$ & $0.898$ & $\pm0.065$ \\ \hline
Logistic & S2 & $0.902$ & $\pm0.070$ & $0.900$ & $\pm0.070$ & $0.900$ & $\pm0.071$ \\ \hline
Gdboosting & S2 & $0.860$ & $\pm0.063$ & $0.854$ & $\pm0.061$ & $0.858$ & $\pm0.067$ \\ \hline
Random forest & S2 & $0.873$ & $\pm0.088$ & $0.880$ & $\pm0.086$ & $0.878$ & $\pm0.091$ \\ \hline
Mult.NB & S1 & $0.853$ & $\pm0.034$ & $0.842$ & $\pm0.034$ & $0.841$ & $\pm0.035$ \\ \hline
Svm & S1 & $0.894$ & $\pm0.045$ & $0.893$ & $\pm0.046$ & $0.893$ & $\pm0.046$ \\ \hline
Logistic & S1 & $0.890$ & $\pm0.048$ & $0.890$ & $\pm0.049$ & $0.890$ & $\pm0.049$ \\ \hline
Gdboosting & S1 & $0.843$ & $\pm0.056$ & $0.843$ & $\pm0.055$ & $0.843$ & $\pm0.055$ \\ \hline
Random forest & S1 & $0.882$ & $\pm0.024$ & $0.876$ & $\pm0.043$ & $0.878$ & $\pm0.039$ \\ \hline
Mult.NB & S4 S3 & $0.851$ & $\pm0.023$ & $0.806$ & $\pm0.036$ & $0.799$ & $\pm0.040$ \\ \hline
Svm & S4 S3 & $0.917$ & $\pm0.021$ & $0.916$ & $\pm0.021$ & $0.916$ & $\pm0.021$ \\ \hline
Logistic & S4 S3 & $0.917$ & $\pm0.019$ & $0.917$ & $\pm0.019$ & $0.917$ & $\pm0.019$ \\ \hline
Gdboosting & S4 S3 & $0.905$ & $\pm0.018$ & $0.905$ & $\pm0.018$ & $0.905$ & $\pm0.018$ \\ \hline
Random forest & S4 S3 & $0.910$ & $\pm0.021$ & $0.908$ & $\pm0.023$ & $0.908$ & $\pm0.024$ \\ \hline
Mult.NB & S4 S2 & $0.872$ & $\pm0.014$ & $0.832$ & $\pm0.025$ & $0.827$ & $\pm0.027$ \\ \hline
Svm & S4 S2 & $0.929$ & $\pm0.011$ & $0.928$ & $\pm0.011$ & $0.928$ & $\pm0.011$ \\ \hline
Logistic & S4 S2 & $0.928$ & $\pm0.011$ & $0.928$ & $\pm0.011$ & $0.928$ & $\pm0.011$ \\ \hline
Gdboosting & S4 S2 & $0.907$ & $\pm0.021$ & $0.907$ & $\pm0.020$ & $0.907$ & $\pm0.020$ \\ \hline
Random forest & S4 S2 & $0.915$ & $\pm0.017$ & $0.914$ & $\pm0.017$ & $0.914$ & $\pm0.020$ \\ \hline
Mult.NB & S4 S1 & $0.853$ & $\pm0.015$ & $0.796$ & $\pm0.026$ & $0.788$ & $\pm0.029$ \\ \hline
Svm & S4 S1 & $0.897$ & $\pm0.014$ & $0.897$ & $\pm0.014$ & $0.897$ & $\pm0.014$ \\ \hline
Logistic & S4 S1 & $0.898$ & $\pm0.014$ & $0.897$ & $\pm0.014$ & $0.897$ & $\pm0.014$ \\ \hline
Gdboosting & S4 S1 & $0.882$ & $\pm0.013$ & $0.883$ & $\pm0.012$ & $0.883$ & $\pm0.013$ \\ \hline
Random forest & S4 S1 & $0.889$ & $\pm0.020$ & $0.887$ & $\pm0.021$ & $0.892$ & $\pm0.024$ \\ \hline
Mult.NB & S3 S2 & $0.781$ & $\pm0.063$ & $0.743$ & $\pm0.056$ & $0.734$ & $\pm0.059$ \\ \hline
Svm & S3 S2 & $0.860$ & $\pm0.050$ & $0.858$ & $\pm0.052$ & $0.858$ & $\pm0.053$ \\ \hline
Logistic & S3 S2 & $0.843$ & $\pm0.048$ & $0.840$ & $\pm0.048$ & $0.839$ & $\pm0.048$ \\ \hline
Gdboosting & S3 S2 & $0.854$ & $\pm0.048$ & $0.849$ & $\pm0.060$ & $0.848$ & $\pm0.060$ \\ \hline
Random forest & S3 S2 & $0.867$ & $\pm0.051$ & $0.861$ & $\pm0.046$ & $0.864$ & $\pm0.048$ \\ \hline
Mult.NB & S3 S1 & $0.820$ & $\pm0.039$ & $0.810$ & $\pm0.042$ & $0.808$ & $\pm0.043$ \\ \hline
Svm & S3 S1 & $0.850$ & $\pm0.034$ & $0.848$ & $\pm0.035$ & $0.848$ & $\pm0.035$ \\ \hline
Logistic & S3 S1 & $0.851$ & $\pm0.040$ & $0.850$ & $\pm0.040$ & $0.849$ & $\pm0.041$ \\ \hline
Gdboosting & S3 S1 & $0.831$ & $\pm0.036$ & $0.834$ & $\pm0.044$ & $0.833$ & $\pm0.044$ \\ \hline
Random forest & S3 S1 & $0.869$ & $\pm0.051$ & $0.872$ & $\pm0.040$ & $0.873$ & $\pm0.050$ \\ \hline
Mult.NB & S2 S1 & $0.848$ & $\pm0.056$ & $0.825$ & $\pm0.064$ & $0.822$ & $\pm0.068$ \\ \hline
Svm & S2 S1 & $0.876$ & $\pm0.041$ & $0.876$ & $\pm0.041$ & $0.876$ & $\pm0.041$ \\ \hline
Logistic & S2 S1 & $0.884$ & $\pm0.042$ & $0.884$ & $\pm0.042$ & $0.884$ & $\pm0.042$ \\ \hline
Gdboosting & S2 S1 & $0.838$ & $\pm0.050$ & $0.837$ & $\pm0.050$ & $0.837$ & $\pm0.051$ \\ \hline
Random forest & S2 S1 & $0.876$ & $\pm0.029$ & $0.876$ & $\pm0.044$ & $0.872$ & $\pm0.039$ \\ \hline
Mult.NB & S4 S3 S2 & $0.862$ & $\pm0.011$ & $0.825$ & $\pm0.016$ & $0.820$ & $\pm0.018$ \\ \hline
Svm & S4 S3 S2 & $0.915$ & $\pm0.019$ & $0.915$ & $\pm0.020$ & $0.915$ & $\pm0.020$ \\ \hline
Logistic & S4 S3 S2 & $0.917$ & $\pm0.016$ & $0.917$ & $\pm0.017$ & $0.917$ & $\pm0.017$ \\ \hline
Gdboosting & S4 S3 S2 & $0.900$ & $\pm0.019$ & $0.900$ & $\pm0.019$ & $0.900$ & $\pm0.019$ \\ \hline
Random forest & S4 S3 S2 & $0.908$ & $\pm0.021$ & $0.907$ & $\pm0.020$ & $0.908$ & $\pm0.023$ \\ \hline
Mult.NB & S4 S3 S1 & $0.844$ & $\pm0.016$ & $0.794$ & $\pm0.025$ & $0.786$ & $\pm0.028$ \\ \hline
Svm & S4 S3 S1 & $0.888$ & $\pm0.015$ & $0.887$ & $\pm0.015$ & $0.887$ & $\pm0.015$ \\ \hline
Logistic & S4 S3 S1 & $0.890$ & $\pm0.015$ & $0.890$ & $\pm0.015$ & $0.890$ & $\pm0.015$ \\ \hline
Gdboosting & S4 S3 S1 & $0.875$ & $\pm0.017$ & $0.875$ & $\pm0.017$ & $0.875$ & $\pm0.017$ \\ \hline
Random forest & S4 S3 S1 & $0.885$ & $\pm0.017$ & $0.888$ & $\pm0.013$ & $0.885$ & $\pm0.014$ \\ \hline
Mult.NB & S4 S2 S1 & $0.862$ & $\pm0.010$ & $0.815$ & $\pm0.017$ & $0.808$ & $\pm0.019$ \\ \hline
Svm & S4 S2 S1 & $0.897$ & $\pm0.014$ & $0.897$ & $\pm0.014$ & $0.897$ & $\pm0.014$ \\ \hline
Logistic & S4 S2 S1 & $0.897$ & $\pm0.015$ & $0.897$ & $\pm0.015$ & $0.897$ & $\pm0.015$ \\ \hline
Gdboosting & S4 S2 S1 & $0.876$ & $\pm0.018$ & $0.876$ & $\pm0.017$ & $0.876$ & $\pm0.018$ \\ \hline
Random forest & S4 S2 S1 & $0.894$ & $\pm0.013$ & $0.891$ & $\pm0.015$ & $0.894$ & $\pm0.015$ \\ \hline
Mult.NB & S3 S2 S1 & $0.832$ & $\pm0.049$ & $0.811$ & $\pm0.056$ & $0.808$ & $\pm0.058$ \\ \hline
Svm & S3 S2 S1 & $0.847$ & $\pm0.039$ & $0.846$ & $\pm0.040$ & $0.846$ & $\pm0.040$ \\ \hline
Logistic & S3 S2 S1 & $0.860$ & $\pm0.035$ & $0.859$ & $\pm0.035$ & $0.859$ & $\pm0.035$ \\ \hline
Gdboosting & S3 S2 S1 & $0.841$ & $\pm0.042$ & $0.841$ & $\pm0.041$ & $0.841$ & $\pm0.042$ \\ \hline
Random forest & S3 S2 S1 & $0.866$ & $\pm0.034$ & $0.867$ & $\pm0.033$ & $0.867$ & $\pm0.038$ \\ \hline
Mult.NB & S4 S3 S2 S1 & $0.854$ & $\pm0.015$ & $0.809$ & $\pm0.023$ & $0.802$ & $\pm0.025$ \\ \hline
Svm & S4 S3 S2 S1 & $0.887$ & $\pm0.020$ & $0.886$ & $\pm0.021$ & $0.886$ & $\pm0.021$ \\ \hline
Logistic & S4 S3 S2 S1 & $0.889$ & $\pm0.023$ & $0.889$ & $\pm0.023$ & $0.889$ & $\pm0.023$ \\ \hline
Gdboosting & S4 S3 S2 S1 & $0.878$ & $\pm0.015$ & $0.878$ & $\pm0.015$ & $0.878$ & $\pm0.016$ \\ \hline
Random forest & S4 S3 S2 S1 & $0.890$ & $\pm0.020$ & $0.887$ & $\pm0.020$ & $0.887$ & $\pm0.014$ \\ \hline
\end{longtable}
\endgroup
\twocolumn
